# Supplementary material for: SA-ConvONet: Sign-Agnostic Optimization of Convolutional Occupancy Networks
Source: arXiv:2105.03582 source file (2021-08-27)
Supplement: Supplementary file 2 [file ablation.tex]

\begin{table}[h]
    %\vspace{-0.3cm}
    
    \setlength{\tabcolsep}{1.5mm}
        \centering
        \scalebox{0.9}{
            \begin{tabular}{l | l |c c c c}
            \toprule
            Datasets & Methods  & CD $\downarrow$ & NC $\uparrow $ & FS ($\tau$) $\uparrow$ &  FS (2$\tau$) $\uparrow$ \\ 
            \hline \hline
             \multirow{2}{*}{\shortstack{ShapaNet \\ -chair~\cite{chang2015shapenet}}}         & opt. enc. &  \textbf{0.516}  &  93.42  &   97.15 &  \textbf{99.40} \\
              & Ours & 0.522 & \textbf{93.51} & \textbf{97.16} & 99.37 \\ 
            \hline
            \multirow{2}{*}{\shortstack{Synethetic \\ Room~\cite{peng2020convolutional}}} & opt. enc. & 0.516  &  89.75  &  93.43  &  98.53 \\
                  & Ours & \textbf{0.495} & \textbf{90.04} &  \textbf{93.85} & \textbf{98.82}   \\
            \hline
            \multirow{2}{*}{ScanNet~\cite{dai2017scannet}}          & opt. enc. & 0.741  & 86.24 & 81.49 & 95.56 \\
               &Ours & \textbf{0.728} & \textbf{86.40} & \textbf{82.08}  & \textbf{95.86}\\
            % \hline
            \bottomrule
            \end{tabular}
        }
        \caption{\textbf{Additional ablation studies} on three datasets.} %The metrics of chamfer distance (CD $\times 0.01$), normal consistency (NC $\times 0.01$), and F-score (FS $\times 0.01$ with the $\tau = 0.01$) are reported.}
        \label{table:ablation}
        \vspace{-5pt}
\end{table}
%\vspace{-0.3cm}
